# Supplementary material for: Symmetries of Chimera States
Source: arXiv:1803.04542 ancillary file (2018-04-26)
Supplement: Supplementary file 1 [file supplement.pdf]

# Supplement - Symmetries of Chimera States

Felix P. Kemeth,[1,2] Sindre W. Haugland,[1,2] and Katharina Krischer[1]

[1] *Physik-Department, Nonequilibrium Chemical Physics, Technische Universität München, James-Franck-Str. 1, D-85748 Garching, Germany*

[2] *Institute for Advanced Study - Technische Universität München, Lichtenbergstr. 2a, D-85748 Garching, Germany*

## AMPLITUDE AND PHASE DIFFERENCE EQUATIONS

The ensemble of four mean-coupled Stuart-Landau oscillators, as described in the main text, can be described by

$$\partial_t W_i = W_i - (1 + ic_2) |W_i|^2 W_i + (\alpha + i\beta) \left( \frac{1}{N} \sum_{j=1}^{N} W_j - W_i \right), \tag{1}$$

with the complex variables $W_i$ and the real parameters $\alpha$, $\beta$ and $c_2$. Hereby, the index $i$ ranges from 1 to 4. By writing $W_i = R_i \exp(i\theta_i)$, the system can be transformed into eight real equations, four for the amplitudes and four for the phases. Due to the rotational invariance of Eq. (1), this can be rewritten as a seven-dimensional system of four amplitude equations and three phase difference equations, which read

$$\begin{aligned}
\partial_t \Delta\theta_{21} = &-c_2 \left( R_2^2 - R_1^2 \right) \\
&+ \frac{\beta}{R_2} \left[ R_1 \cos(\Delta\theta_{21}) + R_3 \cos(\Delta\theta_{32}) + R_4 \cos(\Delta\theta_{43} + \Delta\theta_{32}) \right] \\
&- \frac{\beta}{R_1} \left[ R_2 \cos(\Delta\theta_{21}) + R_3 \cos(\Delta\theta_{32} + \Delta\theta_{21}) + R_4 \cos(\Delta\theta_{43} + \Delta\theta_{32} + \Delta\theta_{21}) \right] \\
&+ \frac{\alpha}{R_2} \left[ R_1 \sin(-\Delta\theta_{21}) + R_3 \sin(\Delta\theta_{32}) + R_4 \sin(\Delta\theta_{43} + \Delta\theta_{32}) \right] \\
&- \frac{\alpha}{R_1} \left[ R_2 \sin(\Delta\theta_{21}) + R_3 \sin(\Delta\theta_{32} + \Delta\theta_{21}) + R_4 \sin(\Delta\theta_{43} + \Delta\theta_{32} + \Delta\theta_{21}) \right] \\
\partial_t \Delta\theta_{32} = &-c_2 \left( R_3^2 - R_2^2 \right) \\
&+ \frac{\beta}{R_3} \left[ R_1 \cos(\Delta\theta_{32} + \Delta\theta_{21}) + R_2 \cos(\Delta\theta_{32}) + R_4 \cos(\Delta\theta_{43}) \right] \\
&- \frac{\beta}{R_2} \left[ R_1 \cos(\Delta\theta_{21}) + R_3 \cos(\Delta\theta_{32}) + R_4 \cos(\Delta\theta_{43} + \Delta\theta_{32}) \right] \\
&+ \frac{\alpha}{R_3} \left[ R_1 \sin(-\Delta\theta_{21} - \Delta\theta_{32}) + R_2 \sin(-\Delta\theta_{32}) + R_4 \sin(\Delta\theta_{43}) \right] \\
&- \frac{\alpha}{R_2} \left[ R_1 \sin(-\Delta\theta_{21}) + R_3 \sin(\Delta\theta_{32}) + R_4 \sin(\Delta\theta_{43} + \Delta\theta_{32}) \right] \\
\partial_t \Delta\theta_{43} = &-c_2 \left( R_4^2 - R_3^2 \right) \\
&+ \frac{\beta}{R_4} \left[ R_1 \cos(\Delta\theta_{43} + \Delta\theta_{32} + \Delta\theta_{21}) + R_2 \cos(\Delta\theta_{43} + \Delta\theta_{32}) + R_3 \cos(\Delta\theta_{43}) \right] \\
&- \frac{\beta}{R_3} \left[ R_1 \cos(\Delta\theta_{32} + \Delta\theta_{21}) + R_2 \cos(\Delta\theta_{32}) + R_4 \cos(\Delta\theta_{43}) \right] \\
&+ \frac{\alpha}{R_4} \left[ R_1 \sin(-\Delta\theta_{43} - \Delta\theta_{32} - \Delta\theta_{21}) + R_2 \sin(-\Delta\theta_{43} - \Delta\theta_{32}) + R_3 \sin(-\Delta\theta_{43}) \right] \\
&- \frac{\alpha}{R_3} \left[ R_1 \sin(-\Delta\theta_{21} - \Delta\theta_{32}) + R_2 \sin(-\Delta\theta_{32}) + R_4 \sin(\Delta\theta_{43}) \right]
\end{aligned}$$

together with the amplitude equations

$$\partial_t R_1 = (1-3\alpha)\, R_1 - R_1^3 + \alpha\left[R_2\cos\left(\Delta\theta_{21}\right) + R_3\cos\left(\Delta\theta_{32}+\Delta\theta_{21}\right) + R_4\cos\left(\Delta\theta_{43}+\Delta\theta_{32}+\Delta\theta_{21}\right)\right]$$
$$- \beta\left[R_2\sin\left(\Delta\theta_{21}\right) + R_3\sin\left(\Delta\theta_{32}+\Delta\theta_{21}\right) + R_4\sin\left(\Delta\theta_{43}+\Delta\theta_{32}+\Delta\theta_{21}\right)\right]$$
$$\partial_t R_2 = (1-3\alpha)\, R_2 - R_2^3 + \alpha\left[R_1\cos\left(\Delta\theta_{21}\right) + R_3\cos\left(\Delta\theta_{32}\right) + R_4\cos\left(\Delta\theta_{43}+\Delta\theta_{32}\right)\right]$$
$$- \beta\left[R_1\sin\left(-\Delta\theta_{21}\right) + R_3\sin\left(\Delta\theta_{32}\right) + R_4\sin\left(\Delta\theta_{43}+\Delta\theta_{32}\right)\right]$$
$$\partial_t R_3 = (1-3\alpha)\, R_3 - R_3^3 + \alpha\left[R_1\cos\left(\Delta\theta_{32}+\Delta\theta_{21}\right) + R_2\cos\left(\Delta\theta_{32}\right) + R_4\cos\left(\Delta\theta_{43}\right)\right]$$
$$- \beta\left[R_1\sin\left(-\Delta\theta_{32}-\Delta\theta_{21}\right) + R_2\sin\left(-\Delta\theta_{32}\right) + R_4\sin\left(\Delta\theta_{43}\right)\right]$$
$$\partial_t R_4 = (1-3\alpha)\, R_4 - R_4^3 + \alpha\left[R_1\cos\left(\Delta\theta_{43}+\Delta\theta_{32}+\Delta\theta_{21}\right) + R_2\cos\left(\Delta\theta_{43}+\Delta\theta_{32}\right) + R_3\cos\left(\Delta\theta_{43}\right)\right]$$
$$- \beta\left[R_1\sin\left(-\Delta\theta_{43}-\Delta\theta_{32}-\Delta\theta_{21}\right) + R_2\sin\left(-\Delta\theta_{43}-\Delta\theta_{32}\right) + R_3\sin\left(-\Delta\theta_{43}\right)\right].$$

## ANALYTIC SOLUTION FOR THE 2-2 CLUSTER STATE

Solutions in which two pairs of two oscillators in the four-oscillator system are synchronized can be obtained analytically, given that they are a fixed point in the amplitude and phase difference variables. Using the fact that this 2-2 cluster state fixed-point solution is also a solution of a system of two mean-coupled oscillators, it is sufficient to find the fixed points of the reduced two-oscillator system

$$\partial_t R_1 = R_1 - R_1^3 + \alpha\left(R_2\cos\left(\Delta\theta\right) - R_1\right) + \beta R_2\sin\left(\Delta\theta\right) \tag{2}$$
$$\partial_t R_2 = R_2 - R_2^3 + \alpha\left(R_1\cos\left(\Delta\theta\right) - R_2\right) - \beta R_1\sin\left(\Delta\theta\right) \tag{3}$$
$$\partial_t \Delta\theta = -c_2\left(R_1^2 - R_2^2\right) + \beta\cos\left(\Delta\theta\right)\left(\frac{R_2}{R_1} - \frac{R_1}{R_2}\right) - \alpha\sin\left(\Delta\theta\right)\left(\frac{R_2}{R_1} + \frac{R_1}{R_2}\right). \tag{4}$$

In addition, these equations can be simplified by introducing the sum and the difference of the squared amplitudes, $\gamma = R_1^2 + R_2^2$ and $\rho = R_1^2 - R_2^2$, with

$$\partial_t\gamma = 2R_1\partial_t R_1 + 2R_2\partial_t R_2$$
$$\partial_t\rho = 2R_1\partial_t R_1 - 2R_2\partial_t R_2.$$

This transforms Eqs. (2) to (4) into

$$\partial_t\gamma = 2\left(1-\alpha\right)\left(R_1^2 + R_2^2\right) - 2\left(R_1^2 + R_2^2\right)^2 + 4R_1^2R_2^2 + 4\alpha R_1R_2\cos\left(\Delta\theta\right)$$
$$\partial_t\rho = 2\left(1-\alpha\right)\left(R_1^2 - R_2^2\right) - 2\left(R_1^4 - R_2^4\right) + 4\beta R_1R_2\sin\left(\Delta\theta\right)$$
$$\partial_t\Delta\theta = -c_2\left(R_1^2 - R_2^2\right) - \beta\cos\left(\Delta\theta\right)\frac{R_1^2 - R_2^2}{R_1R_2} - \alpha\sin\left(\Delta\theta\right)\frac{R_1^2 + R_2^2}{R_1R_2}$$

and using $R_1 R_2 = \sqrt{\gamma^2 - \rho^2}/2$,

$$\partial_t \gamma = 2\left(1-\alpha-\gamma\right)\gamma + \gamma^2 - \rho^2 + 2\alpha\sqrt{\gamma^2-\rho^2}\cos\left(\Delta\theta\right) \tag{5}$$

$$\partial_t \rho = 2\left(1-\alpha-\gamma\right)\rho + 2\beta\sqrt{\gamma^2-\rho^2}\sin\left(\Delta\theta\right) \tag{6}$$

$$\partial_t \Delta\theta = -c_2\rho - 2\beta\cos\left(\Delta\theta\right)\frac{\rho}{\sqrt{\gamma^2-\rho^2}} - 2\alpha\sin\left(\Delta\theta\right)\frac{\gamma}{\sqrt{\gamma^2-\rho^2}}. \tag{7}$$

At a fixed point solution, this system of equations turns into

$$\begin{aligned}
0 &= \left(1-\alpha-\gamma\right)\gamma + \frac{\gamma^2-\rho^2}{2} + \alpha\sqrt{\gamma^2-\rho^2}\cos\left(\Delta\theta\right) \\
0 &= \left(1-\alpha-\gamma\right)\rho + \beta\sqrt{\gamma^2-\rho^2}\sin\left(\Delta\theta\right) \\
0 &= -c_2\rho - 2\beta\cos\left(\Delta\theta\right)\frac{\rho}{\sqrt{\gamma^2-\rho^2}} - 2\alpha\sin\left(\Delta\theta\right)\frac{\gamma}{\sqrt{\gamma^2-\rho^2}}.
\end{aligned}$$

Solving the first two equations for $\cos\left(\Delta\theta\right)$ and $\sin\left(\Delta\theta\right)$ yields

$$\sqrt{\gamma^2-\rho^2}\cos\left(\Delta\theta\right) = -\left(1-\alpha-\gamma\right)\frac{\gamma}{\alpha} - \frac{\gamma^2-\rho^2}{2\alpha} \tag{8}$$

$$\sqrt{\gamma^2-\rho^2}\sin\left(\Delta\theta\right) = -\left(1-\alpha-\gamma\right)\frac{\rho}{\beta} \tag{9}$$

and inserted into the last equation,

$$\begin{aligned}
0 &= -c_2\rho + \frac{\beta}{\alpha}\frac{\rho}{\gamma^2-\rho^2}\left[2\left(1-\alpha-\gamma\right)\gamma + \gamma^2-\rho^2\right] + 2\frac{\alpha}{\beta}\frac{\gamma}{\gamma^2-\rho^2}\left(1-\alpha-\gamma\right)\rho \\
\Rightarrow 0 &= -c_2\left(\gamma^2-\rho^2\right) + \frac{\beta}{\alpha}\left[2\left(1-\alpha-\gamma\right)\gamma + \gamma^2-\rho^2\right] + 2\frac{\alpha}{\beta}\left(1-\alpha-\gamma\right)\gamma \\
\Rightarrow 0 &= -c_2\alpha\beta\left(\gamma^2-\rho^2\right) + 2\beta^2\left(1-\alpha-\gamma\right)\gamma + \beta^2\left(\gamma^2-\rho^2\right) + 2\alpha^2\left(1-\alpha-\gamma\right)\gamma \\
\Rightarrow 0 &= \left(\beta^2 - c_2\alpha\beta\right)\left(\gamma^2-\rho^2\right) + 2\left(\alpha^2+\beta^2\right)\left(1-\alpha-\gamma\right)\gamma.
\end{aligned}$$

Solving for $\rho^2$

$$\rho^2 = 2\frac{\alpha^2+\beta^2}{\beta^2-c_2\alpha\beta}\left(1-\alpha-\gamma\right)\gamma + \gamma^2. \tag{10}$$

Using the identity $1 = \sin^2\left(\Delta\theta\right) + \cos^2\left(\Delta\theta\right)$, we can write Eqs. (8) and (9), yielding

$$\begin{aligned}
\gamma^2-\rho^2 &= \left(1-\alpha-\gamma\right)^2\frac{\rho^2}{\beta^2} + \left(-\left(1-\alpha-\gamma\right)\frac{\gamma}{\alpha} - \frac{\gamma^2-\rho^2}{2\alpha}\right)^2 \\
\Rightarrow \gamma^2-\rho^2 &= \left(1-\alpha-\gamma\right)^2\frac{\rho^2}{\beta^2} + \frac{1}{4\alpha^2}\left(\gamma^2-\rho^2+2\left(1-\alpha-\gamma\right)\gamma\right)^2. \qquad (11)
\end{aligned}$$

By inserting Eq. (10) into Eq. (11), we can solve it for $\gamma$ and obtain

$$\begin{aligned}
\gamma = &\frac{\left(1-\alpha\right)\left(3\beta-4\alpha c_2-\beta c_2^2\right)}{2\beta-4\alpha c_2-2\beta c_2^2} \\
&\pm\frac{\beta\sqrt{\left(1-\alpha\right)^2\left(1+c_2^2\right)^2 - 8\beta^2\left(1-c_2^2\right) + 8\alpha c_2\left(3\beta-2\alpha c_2-\beta c_2^2\right)}}{2\beta-4\alpha c_2-2\beta c_2^2}. \qquad (12)
\end{aligned}$$

Together with Eq. (10), this can be used to calculate $R_1$, $R_2$ and $\Delta\theta$. These expressions then serve as a starting point for a 2-2 cluster solution in the four oscillator system, as described in the main text.

## NUMERICAL METHODS

For the integration of the Stuart-Landau ensemble, an implicit Adams method with a fixed time step of $dt = 0.01$ is used. Initial conditions for the simulations are taken as the 2-2 cluster solution, as given above, with added Gaussian noise of variance $\sigma = 0.01$ and zero mean.

For the simulations of the Ginzburg-Landau equation with one spatial domain, we employed a pseudo-spectral integration method with exponential time-stepping [1] and fixed time step $dt = 0.02$, system size $L = 400$ and $N = 4096$. As boundaries, periodic boundaries were taken. Initial conditions are taken close to the solutions of the symmetric and asymmetric chimera states of the Stuart-Landau ensemble. In particular, we repeated the $W_i$ of the solutions in the minimal chimeras $N/4$ times, and assigned them a spatial coordinate, starting with the values of $W_1$ for small $x$, up to the values of $W_4$ for large $x$. Then we added Gaussian noise of variance $\sigma = 0.01$ and zero mean.

For the Poincaré plot, we used the analytic two-cluster solution at $\alpha = 0.84$, $\beta = -0.8$ as starting point, and subsequently switched the parameters to $\alpha = 0.84$ and $\beta = -0.7$. This ensures that we land on the attractor of interest, which is bistable with the homogeneous solution in this region. We then added Gaussian noise of variance $\sigma = 0.01$ and zero mean, and integrated the system until the initial transients decayed. Subsequently, we integrated the system and record $T = 5{\cdot}10^5$ snapshots between $t_{\text{min}} = 2000$ and $t_{\text{max}} = 7000$, from which we estimated the maxima of the amplitudes. Then, we reduced $\alpha$ in steps of $\Delta\alpha = 5 \cdot 10^{-5}$ and took the last snapshot of the previous integration plus added Gaussian noise of variance $\sigma = 0.01$ and zero mean as initial condition, and repeated the procedure above.

For the calculation of the symmetry detectives, we used $T = 2 \cdot 10^5$ snapshots between $t_{\text{min}} = 1000$ and $t_{\text{max}} = 21000$. All figures are generated using matplotlib [2].

## TIME SERIES OF THE ASYMMETRIC AND SYMMETRIC CHIMERA STATES IN THE MINIMAL AND EXTENDED SYSTEMS

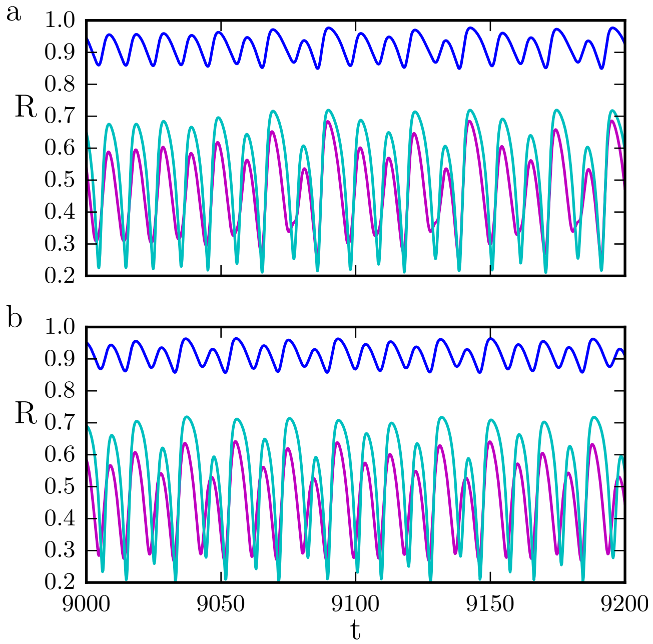


FIG. 1. (a) Time series of the absolute value of $W$ of the asymmetric chimera state in the four oscillator network, as shown in Fig. 2b in the main text. (b) Exemplary time series of the absolute value of $W$ of the asymmetric chimera state in the spatially extended system, at $x = 0$ (magenta), $x = 200$ (blue) and $x = 125$ (cyan), obtained from the data as shown in Fig. 4a in the main text.

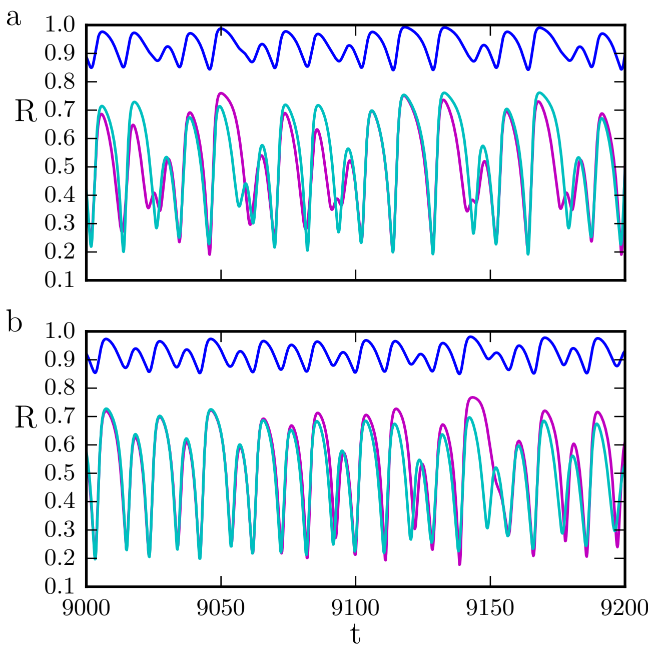


FIG. 2. (a) Time series of the absolute value of $W$ of the symmetric chimera state in the four oscillator network, as shown in Fig. 2d in the main text. (b) Exemplary time series of the absolute value of $W$ of the symmetric chimera state in the spatially extended system, at $x = 0$ (magenta), $x = 200$ (blue) and $x = 75$ (cyan), obtained from the data as shown in Fig. 4b in the main text.

[1] S. Cox and P. Matthews, Journal of Computational Physics **176**, 430 (2002).

[2] J. D. Hunter, Computing In Science & Engineering **9**, 90 (2007).
